# Supplementary material for: On the Prevalence and Usage of Commit Signing on GitHub: A Longitudinal and Cross-Domain Study
Source: arXiv:2504.19215 source file (2025-04-27)
Supplement: Supplementary file 1 [file appendix.tex]

\appendix

\section{Information related to GitHub REST API}

\subsection{States of commit based on commit signature}

\begin{table}[ht]
\caption{Description of different states of commit based on commit signature as per GitHub REST API \cite{githubCommitRest}}
\label{tab:signStatus}
\resizebox{0.9\columnwidth}{!}{%
\rowcolors{1}{white}{gray!25}
\begin{tabular}{@{}ll@{}}
\toprule
Status & Description \\ \midrule
valid & \begin{tabular}[c]{@{}l@{}}The signature is regarded as valid\\as none of the below errors were present.\end{tabular} \\
invalid & \begin{tabular}[c]{@{}l@{}}The signature could not be cryptographically\\ verified using the key whose key-id was\\ found in the signature.\end{tabular} \\
malformed\_signature & There was an error parsing the signature. \\
unknown\_key & \begin{tabular}[c]{@{}l@{}}The key that made the signature has not\\ been registered with any user's account.\end{tabular} \\
bad\_email & \begin{tabular}[c]{@{}l@{}}The committer email address in the\\ commit is not included in the identities\\ of the PGP key that made the signature.\end{tabular} \\
unverified\_email & \begin{tabular}[c]{@{}l@{}}The committer email address in the\\ commit was associated with a user,\\ but the email address is not verified\\ on their account.\end{tabular} \\
no\_user & \begin{tabular}[c]{@{}l@{}}No user was associated with the\\ committer email address in the commit.\end{tabular} \\
unknown\_signature\_type & A non-PGP signature was found in the commit. \\
unsigned & The object does not include a signature. \\
gpgverify\_unavailable & \begin{tabular}[c]{@{}l@{}}The signature verification service is\\ currently unavailable.\end{tabular} \\
gpgverify\_error & \begin{tabular}[c]{@{}l@{}}There was an error communicating with the\\ signature verification service.\end{tabular} \\
not\_signing\_key & \begin{tabular}[c]{@{}l@{}}The "signing" flag is not among the usage\\ flags in the GPG key that made the signature.\end{tabular} \\
expired\_key & The key that made the signature is expired. \\ \bottomrule
\end{tabular}%
}
\end{table}

\input{sections/repo-table}
